# Supplementary material for: System Identification near a Hopf Bifurcation via the Noise-Induced Dynamics in the Fixed-Point Regime
Source: arXiv:2101.06828 source file (2021-01-18)
Supplement: Supplementary file 1 [file appendix1.tex]

%!TEX program = xelatex
%!TEX root = ./thesis.tex
\chapter{Derivation of Fokker--Planck equation with high-order nonlinear terms}

\textit{In this section, we show vdp to FPE (SL?)}

Here we write a Duffing--van der Pol equation with the nonlinearity up to 13th order:

\textit{mention that the number of nonlinear terms can vary}

\begin{equation}\label{a1}
    \ddot{x}-(\epsilon+\alpha_1x^2+\alpha_2x^4+\alpha_3x^6+\alpha_4x^8+\alpha_5x^{10}+\alpha_6x^{12})\dot{x}+x+{\beta}x^3=\sqrt{2d}\eta(t),
\end{equation}
where $\epsilon$ is the linear growth/damping term, $\alpha_n$ terms are nonlinear system parameters, $\beta$ is the anisochronicity factor, $d$ is the noise intensity, and $\eta(t)$ is a Gaussian noise that follows the white noise assumption $\langle\eta(t)\eta(t+\tau)\rangle=\delta(\tau)$ and $\langle\eta(t)\rangle=0$. In order to apply the method of variation of parameters\citep{nayfeh1981introduction,nayfeh1979nonlinear}, we transform the instantaneous state of system ($x(t)$) into amplitude ($a$) and phase ($\phi$):

\begin{subequations}\label{a2}
\begin{align}
    x(t)&=a(t)\cos(\omega t+\phi(t))\label{a2_1},\\
    \dot{x}(t)&=-a(t)\omega\sin(\omega t+\phi(t))\label{a2_2}.
\end{align}
\end{subequations}

Without the loss of generality, we can leave the frequency ($\omega$) at 1. Substituting equation \ref{a1} with equations \ref{a2_1}, \ref{a2_2} and replacing the term $t+\phi(t)$ with $\Phi$, we obtain following set of equations:

\begin{subequations}\label{a3}
\begin{align}
    \dot{a}\cos{\Phi}-a\dot{\phi}\sin{\Phi}=&0 \label{a3_1},\\
    \dot{a}\sin{\Phi}-a\dot{\phi}\cos{\Phi}=&{\epsilon}a\sin{\Phi}+\alpha_{1}a^{3}\sin{\Phi}\cos^2{\Phi}+\alpha_{2}a^{5}\sin{\Phi}\cos^4{\Phi} \notag\\
    &+\alpha_{3}a^{7}\sin{\Phi}\cos^6{\Phi}+\alpha_{4}a^{9}\sin{\Phi}\cos^8{\Phi}+\alpha_{5}a^{11}\sin{\Phi}\cos^{10}{\Phi} \notag \\
    &+\alpha_{6}a^{13}\sin{\Phi}\cos^{12}{\Phi}+{\beta}a^3\cos^3{\Phi}-\sqrt{2d}\eta \label{a3_2}.
\end{align}
\end{subequations}

By multiplying $\cos{\Phi}$ to equation \ref{a3_1} and $\sin{\Phi}$ to equation \ref{a3_2}, we can obtain the following equation for $a'$ is derived by solving the simultaneous equations:

\begin{equation}\label{a4}
\begin{split}
    \dot{a}=&{\epsilon}a\sin^2{\Phi}+\alpha_{1}a^{3}\sin^2{\Phi}\cos^2{\Phi}+\alpha_{2}a^{5}\sin^2{\Phi}\cos^{4}{\Phi}+\alpha_{3}a^{7}\sin^2{\Phi}\cos^{6}{\Phi}\\
    &+\alpha_{4}a^{9}\sin^2{\Phi}\cos^{8}{\Phi}+\alpha_{5}a^{11}\sin^2{\Phi}\cos^{10}{\Phi}+\alpha_{6}a^{13}\sin^2{\Phi}\cos^{12}{\Phi}\\
    &+{\beta}a^3\sin{\Phi}\cos^3{\Phi}-\sqrt{2d}\eta\sin{\Phi}.
\end{split}
\end{equation}

The trigonometric identities can be applied to equation \ref{a4} to remove the exponents of sine and cosine terms. After the arithmetic procedure, equation \ref{a4} can be expressed in the following form:

\begin{equation}\label{a5}
    \dot{a}=\frac{\epsilon}{2}a+\frac{\alpha_1}{8}a^3+\frac{\alpha_2}{16}a^5+\frac{5\alpha_3}{128}a^7+\frac{7\alpha_4}{256}a^9+\frac{21\alpha_5}{1024}a^{11}+\frac{33\alpha_6}{2048}a^{13}+Q_1(\Phi)-(\sqrt{2d}\sin{\Phi})\eta.
\end{equation}

In the equation above, $Q_1(\Phi)$ denotes the sum of all the terms with first-order sine and cosine components (i.e. in the form of $a^{n_1}\cos{n_2\Phi}$). Assuming that a and $\Phi$ vary much slowly than $x$, $Q_1(\Phi)$ become zero on time-averaging. Therefore, for noise-free condition, equation \ref{a5} can be written as:

\begin{equation}\label{a55}
    \dot{a}=\frac{\epsilon}{2}a+\frac{\alpha_1}{8}a^3+\frac{\alpha_2}{16}a^5+\frac{5\alpha_3}{128}a^7+\frac{7\alpha_4}{256}a^9+\frac{21\alpha_5}{1024}a^{11}+\frac{33\alpha_6}{2048}a^{13},
\end{equation}
which takes the form of Stuart--Landau equation.

Similarly, if we multiply $\sin{\Phi}$ to equation \ref{a3_1} and $\cos{\Phi}$ to equation \ref{a3_2}, we obtain the equivalent equation of \ref{a5} for $\dot{\phi}$ as:

\begin{equation}\label{a6}
    \dot{\phi}=\frac{3\beta}{8}a^2+Q_2(\Phi)-\bigg(\frac{\sqrt{2d}}{a}\cos{\Phi}\bigg)\eta,
\end{equation}
where $Q_2(\Phi)$ is also the sum of all terms with first-order cosine components. To apply the stochastic averaging principles, we first divide equations \ref{a5} and \ref{a6} to following set of equations:

\begin{subequations}\label{a7}
\begin{align}
    f_1=\frac{\epsilon}{2}a+\frac{\alpha_1}{8}a^3+\frac{\alpha_2}{16}a^5+\frac{5\alpha_3}{128}a^7+&\frac{7\alpha_4}{256}a^9+\frac{21\alpha_5}{1024}a^{11}+\frac{33\alpha_6}{2048}a^{13}+Q_1(a,\Phi),\\
    f_2&=\frac{3\beta}{8}a^2+Q_2(a,\Phi),\\
    g_1&=\sqrt{2d}\sin{\Phi},\\
    g_2&=\frac{\sqrt{2d}}{a}\cos{\Phi}.
\end{align}
\end{subequations}

Now we can apply the stochastic averaging principles \citep{stratonovich1967,stratonovich1963} to obtain the following It\^o equation of amplitude:

\begin{subequations}\label{a8}
\begin{gather}
\mathrm{d}a=\boldsymbol{m}\mathrm{d}t+\boldsymbol{\sigma}\mathrm{d}W,\\
\boldsymbol{m}=T^{av}\big\{{f_1}\big\}+T^{av}\bigg\{\int_{-\infty}^{0}\Big(\pdv{g_1(s)}{a}g_1(s+\tau)+\pdv{g_1(s)}{\phi}g_2(s+\tau)\Big)\langle\eta(s)\eta(s+\tau)\rangle\mathrm{d}\tau\bigg\}\notag\\
=\frac{{\epsilon}}{2}a+\frac{\alpha_1}{8}a^3+\frac{\alpha_2}{16}a^5+\frac{5\alpha_3}{128}a^7+\frac{7\alpha_4}{256}a^9+\frac{21\alpha_5}{1024}a^{11}+\frac{33\alpha_6}{2048}a^{13}+\frac{d}{2a},\\
\boldsymbol{\sigma}^2=T^{av}\bigg\{\int_{-\infty}^{\infty}g_1(s)g_1(s+\tau)\langle\eta(s)\eta(s+\tau)\rangle\mathrm{d}\tau\bigg\}=d,
\end{gather}
\end{subequations}
where $\mathrm{d}W$ is the unit Wiener process and $T^{av}$ denotes the time average of the functions. The equivalent Fokker-Planck equation is derived as follows:

\begin{equation}\label{a9}
\begin{split}
    \pdv{P(a,t)}{t}=&-\pdv{}{a}\bigg[\Big(\frac{{\epsilon}a}{2}+\frac{\alpha_1a^3}{8}+\frac{\alpha_2a^5}{16}+\frac{5\alpha_3a^7}{128}+\frac{7\alpha_4a^9}{256}+\frac{21\alpha_5a^{11}}{1024}+\frac{33\alpha_6a^{13}}{2048}\\
    &+\frac{d}{2a}\Big)P(a,t)\bigg]+\pdv[2]{}{a}\bigg[\frac{d}{2}P(a,t)\bigg].
\end{split}
\end{equation}

The last term with the second partial derivative is the diffusion term, while the other right-hand side terms are the drift terms. The stationary solution of \ref{a9} is straightforwardly obtained as \ref{a10}.

\begin{equation}\label{a10}
    P(a)=Ca\exp[\frac{a^2}{d}\Big(\frac{\epsilon}{2}+\frac{\alpha_1}{16}a^2+\frac{\alpha_2}{48}a^4+\frac{5\alpha_3}{512}a^6+\frac{7\alpha_4}{1280}a^8+\frac{7\alpha_5}{2048}a^{10}+\frac{33\alpha_6}{14336}a^{12}\Big)].
\end{equation}

It is worth mentioning that the derived stationary Fokker-Planck equation is independent of the anisochronicity factor $\beta$.
